# Supplementary material for: Duet: An Expressive Higher-order Language and Linear Type System for Statically Enforcing Differential Privacy
Source: arXiv:1909.02481 source file (2019-09-05)
Supplement: Supplementary file 1 [file appendix_evaluation.tex]

\begin{table}
  \centering
    \begin{tabular}{r c c c}
    
    \textbf{Dataset} & \textbf{\# Samples} & \textbf{\# Dim.} & \textbf{\# Classes}\\ 
    \hline
    % \multicolumn{4}{c}{\textbf{Public Datasets}}\\
    % \hline
%    Synthetic-L & 10,000 & 20 & 2\\
    Adult & 45,220 & 104 & 2 \\
%    Iris & 150 & 4 & 3 \\
    KDDCup99 & 70,000 & 114 & 2\\
   % Covertype & 581,012 & 54 & 7\\
    Facebook & 40,949 & 54 & 2\\
%~\cite{Facebook-comments}
%    MNIST & 65,000 & 784 & 10\\
    % \hline
    % \multicolumn{4}{c}{\textbf{High-Dimensional Datasets (Public)}}\\
    % \hline
    %Synthetic-H & 2,000 & 2,000 & 2\\
    Gisette & 6,000 & 5,000 & 2\\
%    Real-sim & 72,309 & 20,958 & 2\\
    %RCV1 & 50,000 & 47,236 & 2\\
%    \hline
%    \multicolumn{4}{c}{\textbf{Real-World Datasets (Uber)}}\\
%    \hline
%    Dataset \#1 & 4m & 23 & 2\\
%    Dataset \#2 & 18m & 294 & 2 \\
    % Dataset \#3 & 18m & 20 & 2\\
    % Dataset \#4 & 19m & 70 & 2\\
  \end{tabular}

  \caption{Datasets, with number of samples, number of dimensions,  and number of classes, for algorithm utility evaluation.}
  \label{tbl:datasets_alg}
\end{table}
